# Supplementary material for: Contrastive-mixup learning for improved speaker verification
Source: arXiv:2202.10672 source file (2022-02-22)
Supplement: Supplementary file 1 [file 7_appendix.tex]

\section{Appendix}

\begin{table}[th]
	\caption{Summary statistics of simulation data based on Swithboard and SRE data. Simulation data is used for training EEND, SC-EEND, EDA-EEND models.}
	\label{tab:stats}
	\centering
	\begin{tabular}{r  r r r}
		\toprule
		\multicolumn{1}{c}{\textbf{Speaker \#}} & 
	    \multicolumn{1}{c}{\textbf{\# mixtures}}    &
		\multicolumn{1}{c}{\textbf{Overlap ratio (\%)}} &
		\multicolumn{1}{c}{\textbf{Avg Duration (sec)}}    \\
		\midrule
		1  & 100K & 0.0 &  80 \\
		2  & 100K & 35.2 & 90\\
		3  & 100K & 34.3 & 110\\
		4 & 100K & 30.6  & 128\\
		\bottomrule
	\end{tabular}
\end{table}

@misc{cai2018exploring,
  title={Exploring the Encoding Layer and Loss Function in End-to-End Speaker and Language Recognition System}, 
  author={Weicheng Cai and Jinkun Chen and Ming Li},
  year={2018},
  eprint={1804.05160},
  archivePrefix={arXiv},
  primaryClass={eess.AS}
}

\begin{table}[th]
	\caption{Summary statistics of CALLHOME dataset. We splited CALLHOME data into adaptation and test set using the same recipe in \cite{fujita2019end} to make our results comparable to their results.}
	\label{tab:callhome stats}
	\centering
	\begin{tabular}{ r  r  r  r  }
		\toprule
		\textbf{Speaker \#} &  \textbf{Overall} & \textbf{Adaptation}  & \textbf{Test}  \\ 
		\midrule
		2     & $303$  & $155$ & $148$     \\
		3     & $136$  & $62$ & $74$      \\
		4     & $43$  & $23$ & $20$      \\
		5     &  $10$  & $5$ & $5$     \\
		6      & $6$  & $3$ & $3$    \\
		7      & $2$   & $2$ & $0$      \\
		\hline
		Total& $500$   & $250$ & $250$      \\
		\bottomrule
	\end{tabular}

	\begin{tabular}{ r  r  r  r  }
	\toprule
	\textbf{Speaker \#} &  \textbf{Overlap ratio (\%)} & \textbf{Avg Duration (sec)}  \\ 
	\midrule
	2     & $13.54$  & $73.10$     \\
	3     & $18.08$  & $135.68$       \\
	4     & $16.88$  & $329.80$       \\
	5     &  $18.66$  & $384.05$     \\
	6      & $28.19$  & $429.89$    \\
	7      & $30.52$   & $525.26$     \\
	\bottomrule
\end{tabular}
\end{table}

%-----------------------------------------------------------------------------------------------------------------------%
